# Supplementary material for: ParSEL: Parameterized Shape Editing with Language
Source: arXiv:2405.20319 source file (2024-05-31)
Supplement: Supplementary file 1 [file tab_dsl.tex]

\begin{table*}[t!]
    \centering
    \begin{tabular}{lcc}
        \toprule
         Edit Operators & Instantiation & Algebraic Form\\
        \midrule
        \midrule
        \textsc{Translate} &
        \texttt{translate($\mathbf{H}_i$, dir=$\mathbf{n}$, amt=$x$)} &
        $
        \mathbf{H}_i(x) = \mathbf{H}_i^0 + x \cdot \mathbf{n}
        $
        \\
        \midrule
        \textsc{Rotate} &
        \texttt{rotate($\mathbf{H}_i$, orig=$\mathbf{o}$, axis=$\mathbf{n}$, amt=$x$)} &

        \(
        \begin{array}{r@{\;}c@{\;}l}
        \mathbf{R}(x)&=&\cos(x) \mathbf{I} + \sin(x) [\mathbf{n}]_{\times} 
         +  (1 - \cos(x)) \mathbf{n} \mathbf{n}^T\\
        \mathbf{H}_i(x)&=&\mathbf{o} + \mathbf{R}(x) (\mathbf{H}_i^0 - \mathbf{o})
        \end{array}
        \)
        \\
        \midrule
        \textsc{Scale1D} &
        \texttt{scale\_1D($\mathbf{H}_i$, orig=$\mathbf{o}$, dir=$\mathbf{n}$, amt=$x$)} &
        $
        \mathbf{H}_i(x) = \mathbf{o} + x (\mathbf{n} \cdot (\mathbf{H}_i^0 - \mathbf{o})) \mathbf{n} + (\mathbf{H}_i^0 - \mathbf{o})
        $
        \\
        \midrule
        \textsc{Scale2D} &
        \texttt{scale\_2D($\mathbf{H}_i$, orig=$\mathbf{o}$, normal=$\mathbf{n}$, amt=$x$)} &
        \(
        \begin{array}{r@{\;}c@{\;}l}
        \mathbf{H}_i^c  &=& \mathbf{H}_i^0 - \mathbf{o} \\
        \mathbf{H}_i^p  &=& \mathbf{H}_i^c - (\mathbf{H}_i^c \cdot \mathbf{n}) \mathbf{n}\\
        \mathbf{H}_i(x)  &=& \mathbf{o} + (1 + x) \mathbf{H}_i^p + (\mathbf{H}_i^c \cdot \mathbf{n}) \mathbf{n}
        \end{array}
        \)
        \\
        \midrule
        \textsc{Scale3D} &
        \texttt{scale\_3D($\mathbf{H}_i$, orig=$\mathbf{o}$, amt=$x$)} &
        $
        \mathbf{H}_i(x) = \mathbf{o} + (1 + x) (\mathbf{H}_i^0 - \mathbf{o})
        $
        \\
        \midrule
        \textsc{Shear} &
        \texttt{shear($\mathbf{H}_i$, orig=$\mathbf{o}$,
        normal=$\mathbf{n}$,
        dir=$\mathbf{d}$,
        amt=$x$)} 
        &
        \(
        \begin{array}{r@{\;}c@{\;}l}
        \mathbf{H}_i^c  &=& \mathbf{H}_i^0 - \mathbf{o} \\
        \mathbf{S}  &=& \mathbf{I} + x \mathbf{d} \otimes \mathbf{n} \\
        \mathbf{H}_i(x)  &=& \mathbf{o} + \mathbf{S}^T \mathbf{H}_i^c
        \end{array}
        \)
        \\
        \midrule
        \textsc{ChangeCount} 
        &
        \texttt{change\_count($SymR_i$, amt=$x$)}
        &
        -
        \\
        \midrule
        \textsc{ChangeDelta} &
        \texttt{change\_delta($SymR_i$, amt=$x$)} & -
        \\
        \midrule 
        \textsc{KeepFixed} 
        &
        \texttt{keep\_fixed($\mathbf{H}_i$)} 
        &
         $\mathbf{H}_i(x) = \mathbf{H}_i^0 $
        \\
        \bottomrule
    \end{tabular}
    \caption{
    \textbf{DSL commands}:
    We enlist the parameterized editing operators provided in our DSL. Each command is parameterized by a variable $x$, which controls the edit magnitude. We omit the algebraic form of the \textsc{ChangeCount} and \textsc{ChangeDelta}, the two operators which are applied on symmetry relations due to their complexity.
    Note that the initial 6 operators can also be applied only on part features such as a face, edge or a vertex, enabling non-affine transforms.
    }
    \label{tab:dsl}
\end{table*}
