# Supplementary material for: ParSEL: Parameterized Shape Editing with Language
Source: arXiv:2405.20319 source file (2024-05-31)
Supplement: Supplementary file 2 [file tab_relations.tex]

\begin{table*}[t!]
    \centering
    \begin{tabular}{lcc}
        \toprule
         Relation & Instantiation & Constraint\\
        \midrule
        \textsc{ReflectionSymmetry} & 
        \texttt{ref\_sym($\mathbb{H}$, origin=$\mathbf{o}$, normal=$\mathbf{n}$)} &
        $
        || \mathbf{H}_j - \mathbf{H}_i - 2 \left( (\mathbf{H}_i - \mathbf{o}) \cdot \mathbf{n} \right) \mathbf{n}||_\infty < \delta \, \forall \, \mathbf{H}_i, \mathbf{H}_j \in \mathbb{H}
        $
        \\
        \textsc{RotationSymmetry} &
        \texttt{rot\_sym($\mathbb{H}$, point=$\mathbf{o}$, rot\_mat=$\mathbf{R}$)} &
        $
        || \mathbf{H}_j - \mathbf{o} + \mathbf{R}^n (\mathbf{H}_i - \mathbf{o}) ||_\infty < \delta \, \forall \, \mathbf{H}_i, \mathbf{H}_j \in \mathbb{H}, n = i - j 
        $
        \\
        \textsc{TranslationSymmetry} &
        \texttt{trans\_sym($\mathbb{H}$, delta=$\mathbf{d}$)} &
        $
        || \mathbf{H}_j - (\mathbf{H}_i + \mathbf{d}) ||_\infty < \delta \, \forall \, \mathbf{H}_i, \mathbf{H}_j \in \mathbb{H}, n = i - j 
        $
        \\
        \midrule
        \textsc{PointAttachment} & 
        \texttt{point\_attach($\mathbb{A}$, $\mathbb{B}$)} &
        $
        || M_{a} \mathbf{H}_i - M_{b} \mathbf{H}_j ||_\infty < \delta \, \forall \, a_n \in \mathbb{A}, b_n \in \mathbb{B}
        $
        \\
        \textsc{LineAttachment} &
        \texttt{line\_attach($\mathbb{A}$, $\mathbb{B}$)} &
        $
        || M_{a_n} \mathbf{H}_i - M_{b_n} \mathbf{H}_j ||_\infty < \delta \, \forall \, a_n \in \mathbb{A}, b_n \in \mathbb{B}, 
        \{ n \in \mathbb{Z} \mid 1 \leq n \leq 2 \}
        $\\
        \textsc{FaceAttachment} &
        \texttt{face\_attach($\mathbb{A}$, $\mathbb{B}$)} &
        $
        || M_{a_n} \mathbf{H}_i - M_{b_n} \mathbf{H}_j ||_\infty < \delta \, \forall \, a_n \in \mathbb{A}, b_n \in \mathbb{B}, 
        \{ n \in \mathbb{Z} \mid 1 \leq n \leq 4 \}
        $\\
        \textsc{VolumeAttachment} &
        \texttt{vol\_attach($\mathbb{A}$, $\mathbb{B}$)} &
        $
        || M_{a_n} \mathbf{H}_i - M_{b_n} \mathbf{H}_j ||_\infty < \delta \, \forall \, a_n \in \mathbb{A}, b_n \in \mathbb{B}, 
        \{ n \in \mathbb{Z} \mid 1 \leq n \leq 8 \}
        $\\
        \bottomrule
    \end{tabular}
    \caption{
    \textbf{Inter-Part Relations}:
    We enlist the different inter-part relations supported in our structured shape representation. In the first column, we annotate the type of each relation. The second column depicts the pseudo-code used to initialize these relations, providing reference for the relation parameters. Finally, the last column depicts the constraints that are enforced as a consequence of each relation. Note that for the Attachment relations, $M_i$ denotes the harmonic coordinates~\cite{harm_coords} for the corresponding point $i$.
    }
    \label{tab:relations}
\end{table*}
