# Supplementary material for: ParSEL: Parameterized Shape Editing with Language
Source: arXiv:2405.20319 source file (2024-05-31)
Supplement: Supplementary file 3 [file fig_percept_failure.tex]

\begin{figure}
    \centering
    \includegraphics[width=1.0\linewidth]{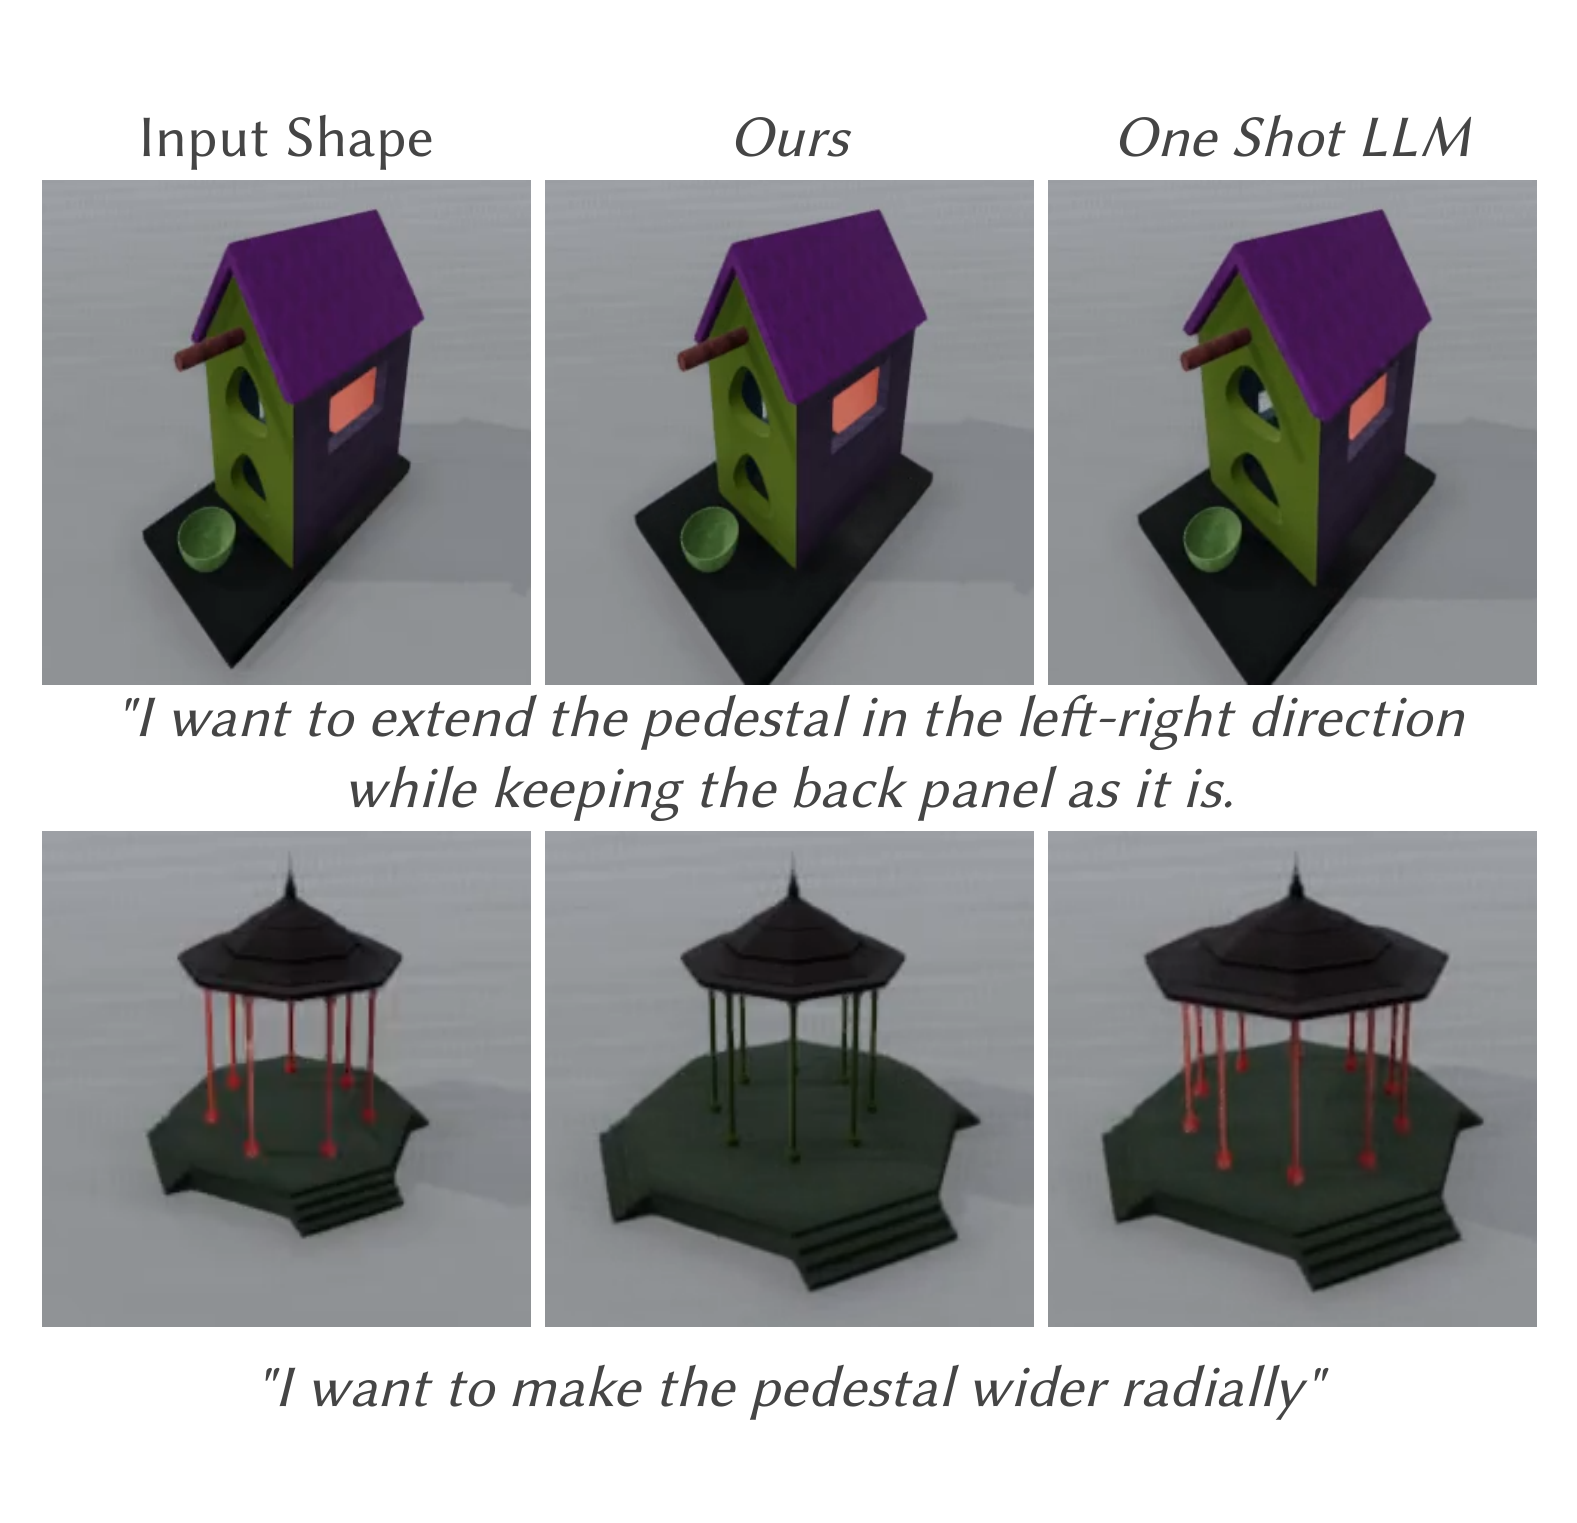}
    \caption{
    \textbf{Perceptual Study Analysis}: In a few cases, as shown above, users preferred \textit{One Shot LLM} over \textit{Ours}. 
    We note that this preference is not caused by a \textit{Ours}'s failure to infer a valid program, but a misalignment between the system interpretation (perform secondary adjustments) and the participant's interpretation (do not perform any secondary adjustments).
    }
    % \vspace{-1.25em}
    \label{fig:percept_failure}
\end{figure}
