# Supplementary material for: ParSEL: Parameterized Shape Editing with Language
Source: arXiv:2405.20319 source file (2024-05-31)
Supplement: Supplementary file 4 [file fig_percept_interface.tex]

\begin{figure}
    \centering
    \includegraphics[width=1.0\linewidth]{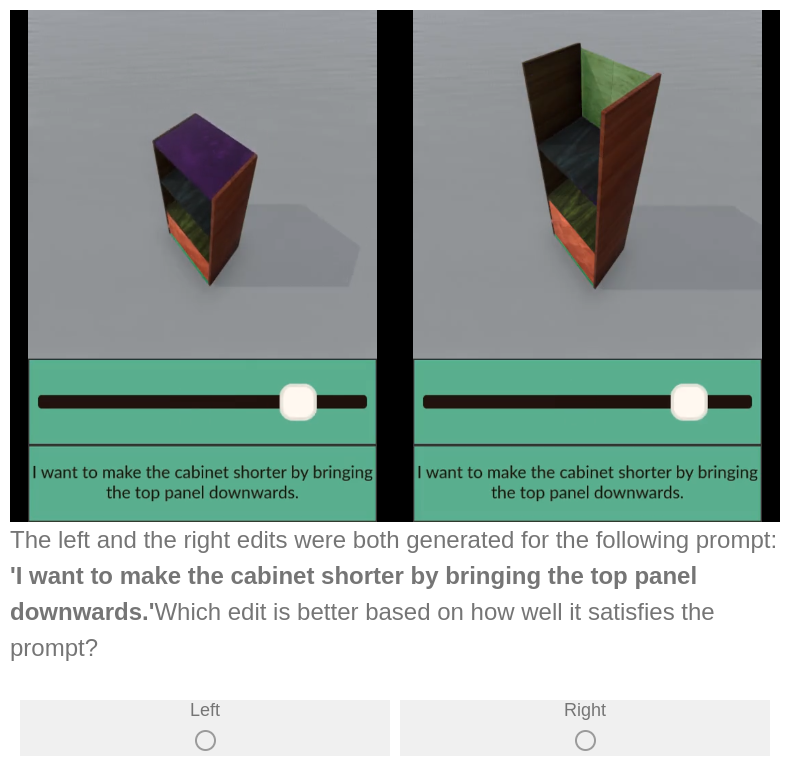}
    \caption{
    \textbf{Perceptual Study Interface}: We provide a screenshot of the questionnaire provided to the participants in our two-alternatives forced-choice perceptual study.
    Note that the videos used for this study are provided in the supplemental material.
    }
    \label{fig:percept_interface}
\end{figure}
