# Supplementary material for: ParSEL: Parameterized Shape Editing with Language
Source: arXiv:2405.20319 source file (2024-05-31)
Supplement: Supplementary file 5 [file fig_recon.tex]

\begin{figure*}
    \centering
    \includegraphics[width=1.0\linewidth]{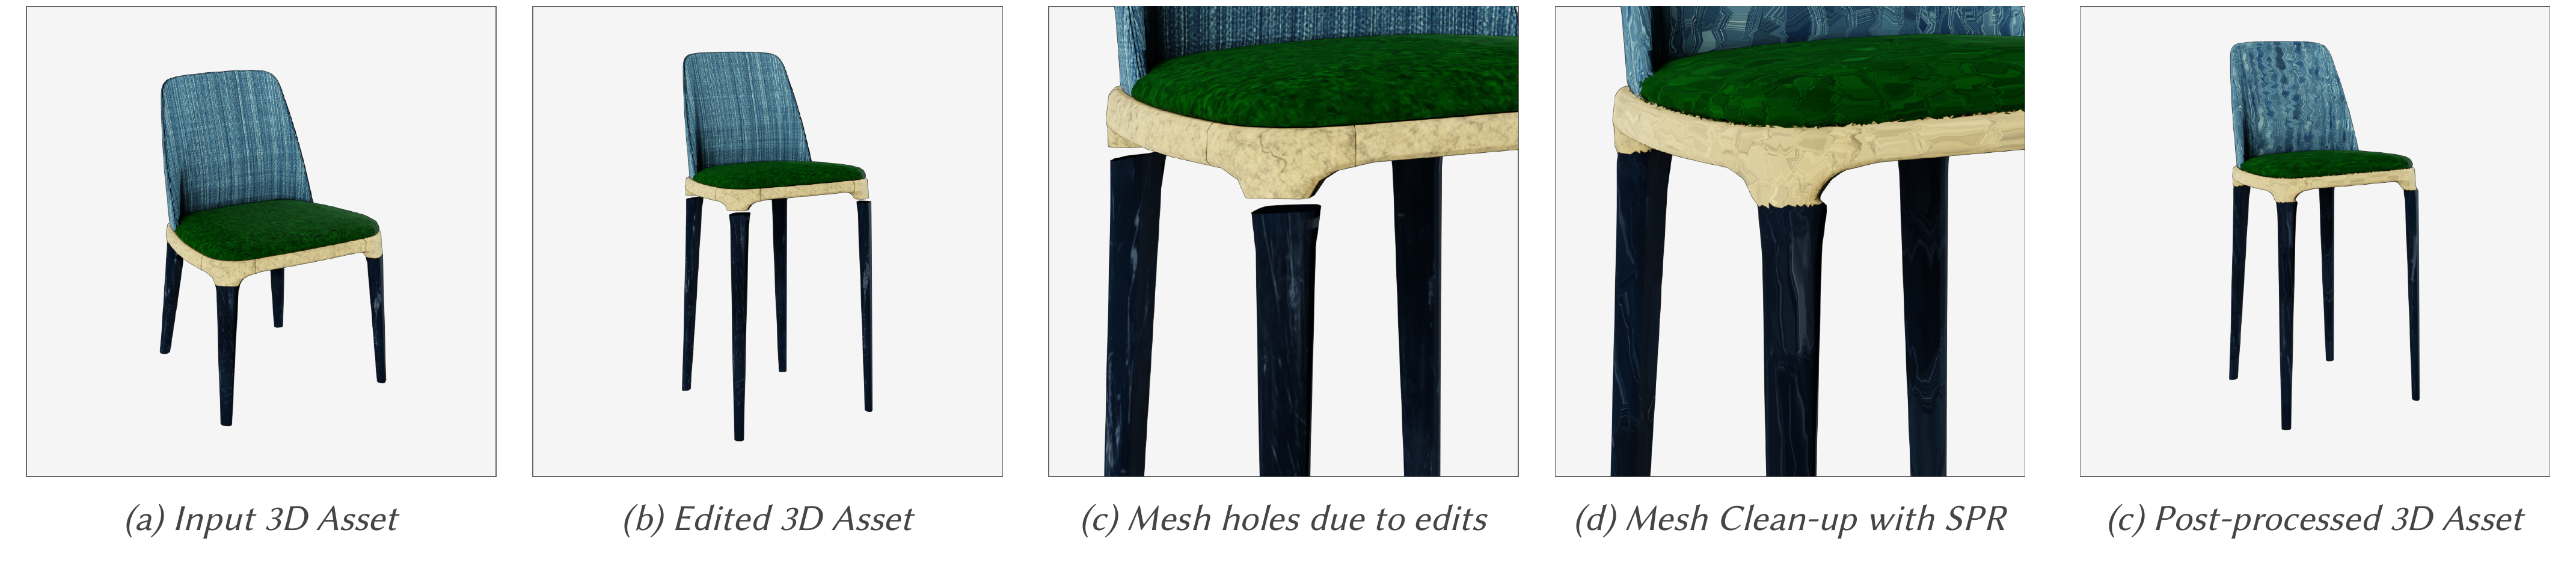}
    \caption{
    \textbf{Perceptual Study Interface}: Extreme deformation under our system can cause gaps to appear in the 3D mesh. With the post-processing we describe in Section~\ref{sec:post-processing}, which employs screened Poisson surface reconstruction (SPR)~\cite{spr}, these gaps can be fixed although with a detrimental effect on the shape's material.
    }
    \label{fig:recon}
\end{figure*}
