# Supplementary material for: ParSEL: Parameterized Shape Editing with Language
Source: arXiv:2405.20319 source file (2024-05-31)
Supplement: Supplementary file 6 [file tab_dataset.tex]

\begin{table*}[t!]
    \centering
    \begin{tabular}{lcccccccccc}
        \toprule
         \multirow{2}{*}{Dataset} & \multirow{2}{*}{N. Shapes} & \multicolumn{3}{c}{N. Parts} & \multicolumn{3}{c}{N. Attachment Relations} & \multicolumn{3}{c}{N. Symmetry Relations} \\
         && Min & Mean & Max & Min & Mean & Max & Min & Mean & Max \\
        \midrule
        PartNet Lamp & 7& 5 & 11.57 & 30 & 4 & 7.00 & 12 & 0 & 1.71 & 4 \\
        PartNet Chair & 15& 7 & 16.40 & 31 & 2 & 18.93 & 42 & 1 & 5.60 & 11 \\
        PartNet Table & 9&5 & 12.89 & 20 & 3 & 14.44 & 41 & 1 & 6.22 & 16 \\
        PartNet Storage Furniture & 13& 12 & 21.67 & 48 & 17 & 51.83 & 117 & 3 & 8.50 & 18\\
        PartNet Bed & 7&17 & 44.25 & 81 & 31 & 77.25 & 110 & 7 & 24.88 & 53\\
        \midrule
        PartNet (\textit{dev-set}) & 51 & 5 & 19.5& 81& 2& 31.82& 117& 0&7.96 & 42 \\
        \midrule
        CoMPaT3D++ (\textit{test-set}) & 50& 3& 12.5& 23& 1& 19.54& 72& 0& 4.8 & 14 \\
        \bottomrule
    \end{tabular}
    \caption{
    \textbf{Dataset Statistics}: We provide statistics of the two datasets we use. We note that our \textit{dev-set}, explores a wider range of structural complexity, whereas our \textit{test-set} explores a wider range of semantic variations (as it contains shape from 21 different categories).
    }
    \label{tab:dataset}
\end{table*}
